# Supplementary material for: Molecular simulations matching denaturation experiments for N6-Methyladenosine
Source: arXiv:2203.14886 ancillary file (2022-05-02)
Supplement: Supplementary file 1 [file SI.pdf]

# Molecular simulations matching denaturation experiments for N6-Methyladenosine

Valerio Piomponi, Thorben Froehlking, Mattia Bernetti, Giovanni Bussi

May 2, 2022

## S1 Parameters adapted from Aduri et al.

Before reparametrizing charges using alchemical calculations, we adapted the Aduri et al. parameters [1] to the current AMBER force field [2, 3, 4]. In particular, we used backbone charges from the current AMBER force field combined with the original Aduri et al. parameters, adding a correction spread on all atoms so as to preserve the correct charge of the nucleotide. Charges are reported in Table S2. We then considered the parametrization of the angle  $\eta_6$ , defined by the atoms N1-C6-N6-C10. We performed a well-tempered metadynamics calculation [5] using  $\eta_6$  as a collective variable. Metadynamics was performed using the PLUMED package [6], with a simulation length of 100 *ns*, depositing a Gaussian every 500 time steps, with initial height equal to 1.2 *kJ/mol* and width  $\sigma = 0.35$ . The Bias factor was set to 10. We then used the free energy profile computed along  $\eta_6$  (see Fig. S1) to estimate the  $\Delta G_{syn/anti}$  by integrating over the two corresponding minima. The result is  $\Delta G_{syn/anti} = 1.5$  *kJ/mol*, which is an underestimation with respect to the experimental value 6.3 *kJ/mol*. We thus decided to add to the potential a single torsional term in this form

$$U(x_i) = \frac{V_\eta}{2} [1 + \cos(\eta_6(x_i) - \pi)] \quad (1)$$

For positive value of the parameter  $V_\eta$  this correction penalizes the *anti* conformations. We then used the MetaD trajectory and obtained biases in a reweighting scheme, tuning the parameter  $V_\eta$  in order to enforce the experimental value of  $\Delta G_{syn/anti}$ . Specifically, we assigned a weight  $w(x)$  to each frame, computed as

$$w(x) \propto e^{\beta B(\eta_6(x))} e^{-\beta \frac{V_\eta}{2} [1 + \cos(\eta_6(x) - \pi)]} \quad (2)$$

Here  $B(\eta_6)$  is the bias potential constructed during MetaD simulation and dependent on time.

The  $\Delta G_{syn/anti}$  was then obtained as

$$\Delta G_{syn/anti} = -\frac{1}{\beta} \log \left( \frac{\sum_{x \in syn} W(x)}{\sum_{x \in anti} W(x)} \right) \quad (3)$$

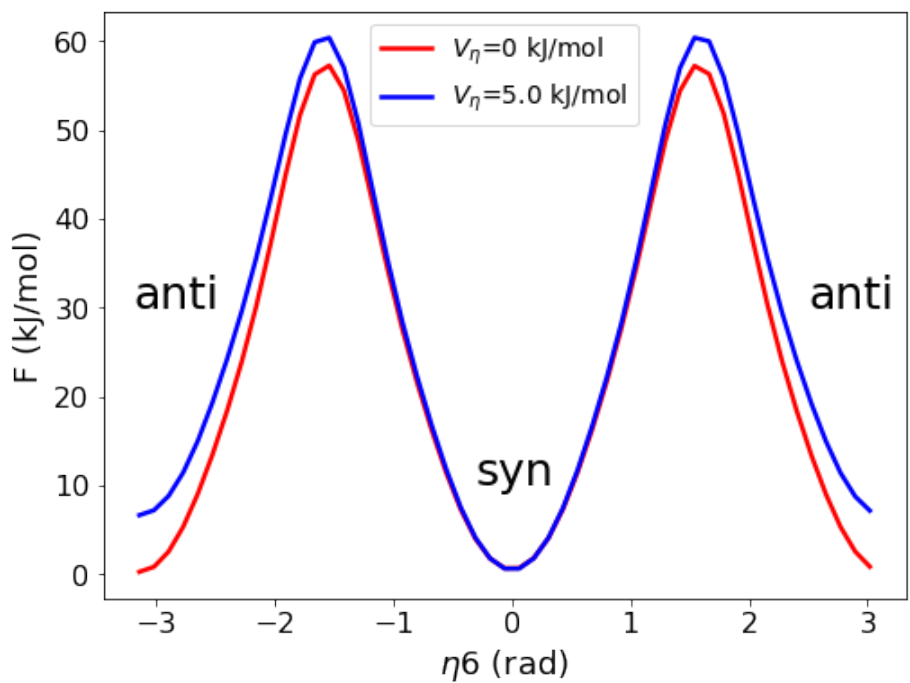

Figure S1: Free Energy Profiles along  $\eta_6$  reconstructed using Metadynamics along the collective variable  $\eta_6$ . The red line corresponds to the profile obtained with the standard Aduri parametrization ( $V_\eta = 0$  kJ/mol), whereas the blue line corresponds to the one obtained with Aduri+tors parametrization ( $V_\eta = 5$  kJ/mol)

We iteratively adjusted  $V_\eta$  until we found that  $V_\eta = 5.0 \text{ kJ/mol}$  results in a  $\Delta G_{syn/anti} = 6.4 \pm 0.3 \text{ kJ/mol}$ , which is compatible with experiment. Statistical error was computed using block analysis [5]. Figure S1 shows the Free Energy profiles reconstructed along  $\eta 6$  for  $V_\eta = 0$  (reference) and  $V_\eta = 5.0 \text{ kJ/mol}$ .

|             | 0   | 1    | 2    | 3    | 4    | 5   | 6    | 7    | 8    | 9    | 10  | 11   | 12   | 13   | 14   | 15  |
|-------------|-----|------|------|------|------|-----|------|------|------|------|-----|------|------|------|------|-----|
| <b>set1</b> | 0.0 | 0.01 | 0.03 | 0.05 | 0.10 | 0.2 | 0.35 | 0.45 | 0.55 | 0.65 | 0.8 | 0.9  | 0.95 | 0.97 | 0.99 | 1.0 |
| <b>set2</b> | 0.0 | 0.02 | 0.05 | 0.09 | 0.14 | 0.2 | 0.3  | 0.43 | 0.57 | 0.7  | 0.8 | 0.86 | 0.91 | 0.95 | 0.98 | 1.0 |

Table S1: Sets of lambda coefficients used in AFEC replica exchange simulations for systems with a single methylation (set 1) or with two methylations (set 2).

## S2 $\lambda$ Spacing

An important choice in setting up alchemical free-energy calculations (AFECs) is the number of intermediate steps and the optimal values for the  $\lambda$  variable. In a replica-exchange setting, the acceptance rate can be used as a measure of the phase-space overlap between adjacent ensembles. A minimum acceptance is then required to enable mixing of ensembles. At the same time, the spacing in  $\lambda$  required to reach this minimum acceptance might differ in different regions of the  $\lambda$  space, thus leading to an optimal allocation of replicas that is not uniformly spaced in  $\lambda$ . We here used a single system, that is the *stand alone* nucleoside in solution, to optimize this ladder and then recycled the same parameters for all systems. Specifically, we empirically adjusted the  $\lambda$  values until we obtained a set of 16 intermediates (set1 in table S1) leading to an approximately uniform acceptance rate (Figure S2), each of them greater than 20%. As it can be seen, the density of the chosen  $\lambda$  values is inhomogenous and, in particular, higher close to the boundaries ( $\lambda = 0$  or 1). This set of lambdas was then used for all the AFECs presented in this work where a single adenine is methylated, and as expected lead to an acceptance greater than 20% for most replica pairs, and greater than 10% for all replica pairs. In cases where two methylations were included (systems B2 to B5 in table 1 of main text), we found that for some pairs of replicas the acceptance was significantly lower than 20%. We notice that in principle the presence of two simultaneous methylation should lead to a larger number of replicas required to obtain the same acceptance. We notice however that some of the acceptances reported in Fig. S2 are significantly larger than 20%. By reoptimizing the parameters, we obtained a set of 16  $\lambda$ 's (set 2 in Table S1) that was able to guarantee an acceptance greater than 20% for all transitions in systems with two methylations.

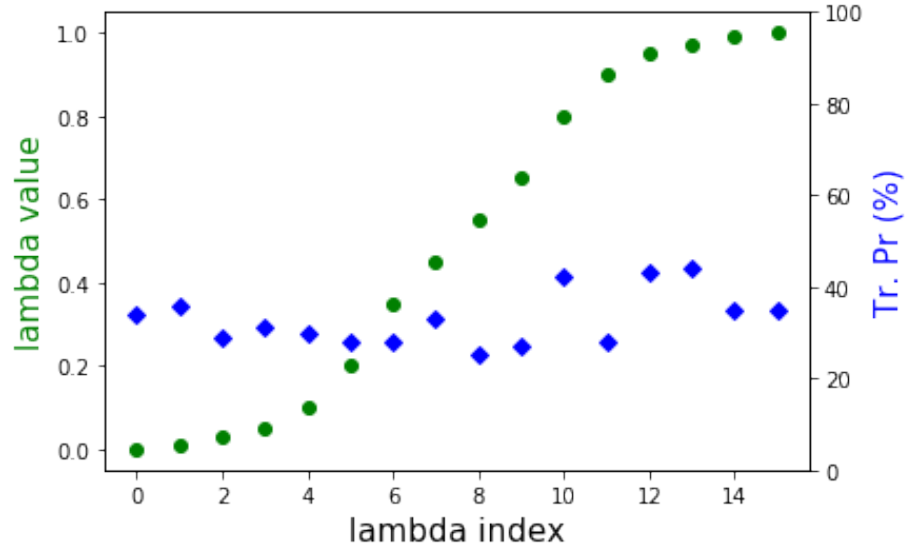

Figure S2: set1  $\lambda$  values (green circles) and transition probabilities in HREX between replica  $\lambda_i$  and  $\lambda_{i+1}$  (blue squares) as a function of  $\lambda$  index  $i$ .

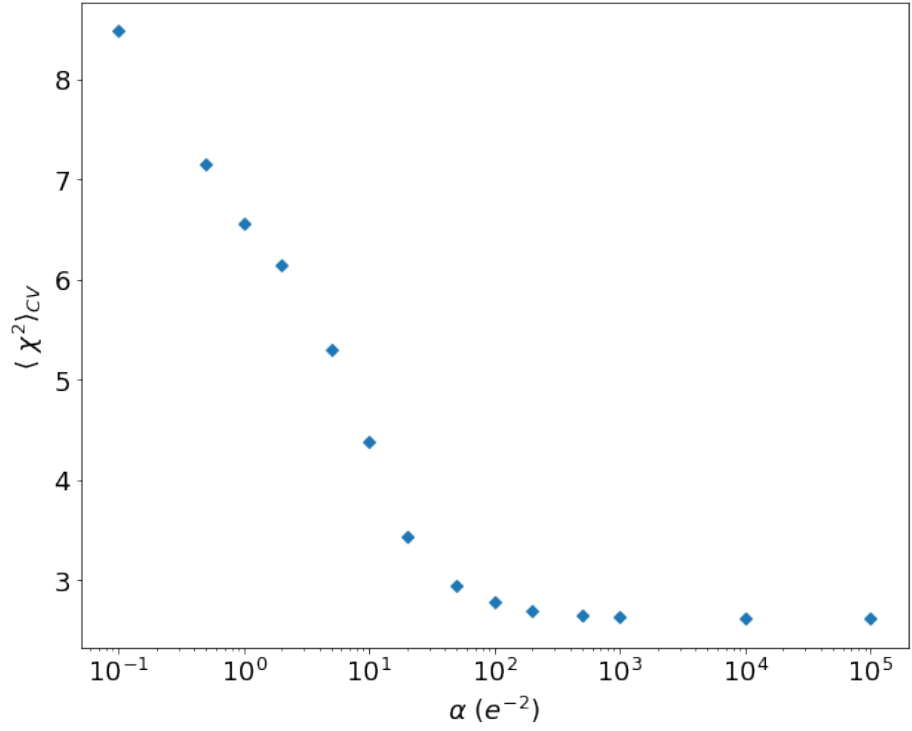

Figure S3: Cross Validation with Leave One Out procedure in fit\_A. Projection of data in plot of Fig. 3a in main text along  $\beta = 0$ .

### S3 Cross validation details

We here report the results of the cross-validation procedure as a function of the hyper-parameter  $\alpha$  (regularization on charges), by keeping the hyper-parameter  $\beta = 0$  (regularization on torsional potential). Results for the fitting on the smaller dataset (fit\_A) are reported in Fig. S3. Results for the fitting on the larger dataset (fit\_AB) are reported in Fig. S4.

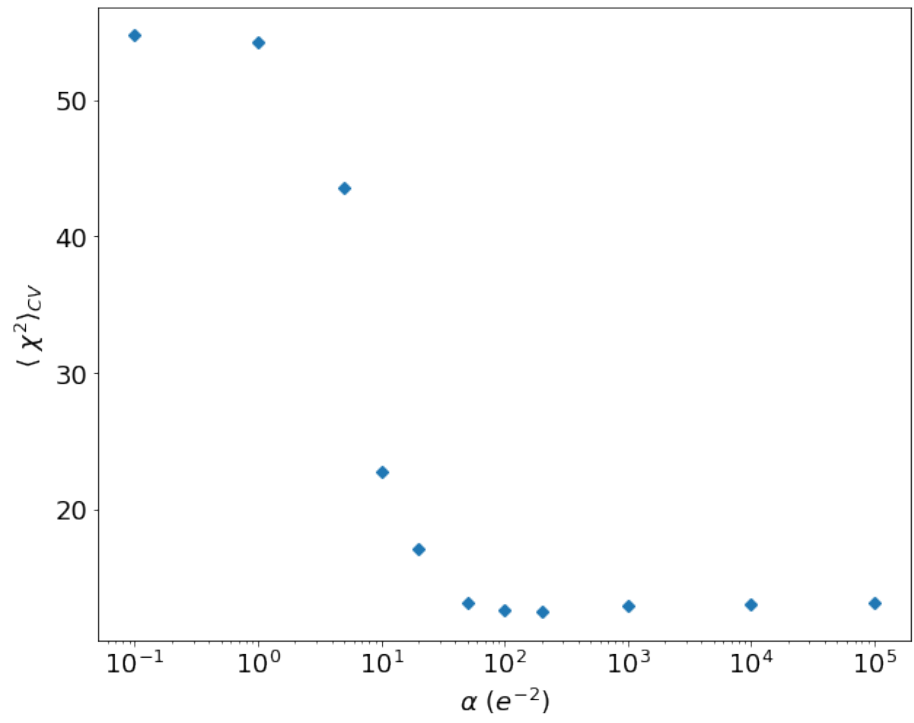

Figure S4: Cross Validation with Leave One Out procedure in fit\_AB. Projection of data in plot of Fig. 4a in main text along  $\beta = 0$ .

## S4 Fit\_A\_incorrect

Fit\_A\_incorrect is a set of parameters that we obtained at an intermediate step of this work. Specifically, in an initial version of our code, the modification of the charge for atom C6 was obtained as the negative of the modifications on the other atoms, so as to maintain the total charge, but it was incorrectly excluded from the regularization term. As it can be seen in Figure S5, the charge modification associated to C6 is larger than those associated to the other atoms in the limit of large  $\alpha$ , as expected as a consequence of this mistake. We then performed new optimizations where the regularization term was correctly including all charges, as reported in the main text. However, the simulations obtained with this incorrect set of charges were used in the analysis. Indeed, this set of charges is closer to the correctly optimized ones with respect to the initial Aduri et al. charges, and thus lead to a larger statistical significance on the computations made for validating *alpha* values in the main text.

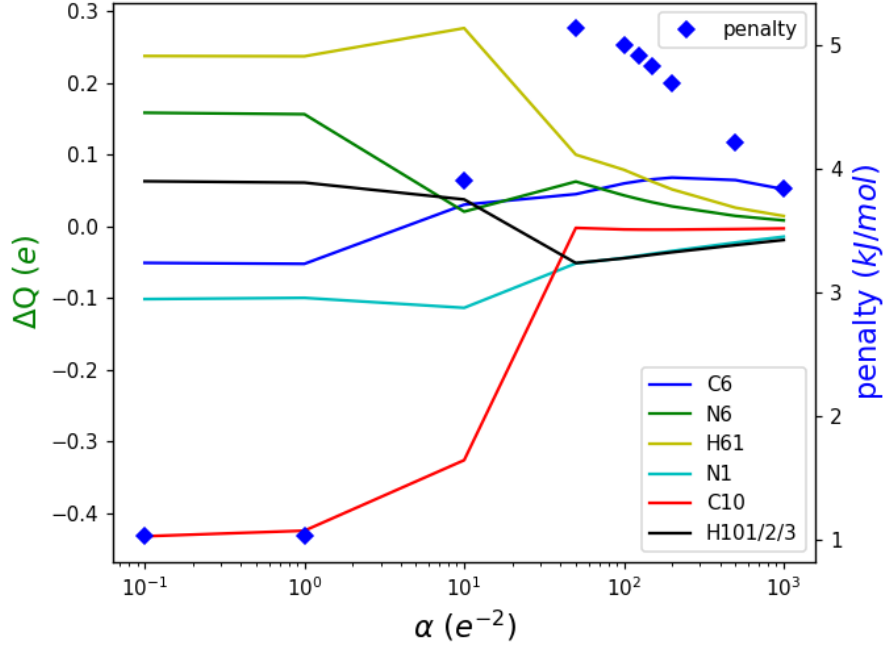

Figure S5: Parameters ( $\Delta Q$  and  $V_\eta$ ) obtained from the entire initial dataset (A) as a function of  $\alpha$ , with  $\beta = 0$ . In this case the fitting was performed as the one shown in Fig. 3 of the main text, but with a missing regularization on the charge of the atom C6 of m6A. From this fitting we derived a parametrization, selecting  $\alpha = 125 e^{-2}$ , which we refer to as `fit_A_incorrect`. Trajectories run with this parametrization were used to compute free energies shown in Fig. 3d of the main text through a reweighting procedure. Another minor difference with respect to the results reported in Fig. 3 was that here the effect of the torsional potential was indirectly computed by adding an energy  $\sim 2V_\eta$  to the *anti* conformation, rather than with a reweighting of the added cosine function. In this figure, we directly report the value of the penalty  $\sim 2V_\eta$ .

|      | Aduri    | fit_A_inc | fit_A    | fit_AB   | RESP_anti | RESP_syn | Krepl   |
|------|----------|-----------|----------|----------|-----------|----------|---------|
| N9   | -0.07829 | -0.07829  | -0.07829 | -0.07829 | -0.0564   | -0.1834  | -0.1719 |
| C8   | 0.13844  | 0.13844   | 0.13844  | 0.13844  | 0.0815    | 0.2573   | 0.0631  |
| H8   | 0.16681  | 0.16681   | 0.16681  | 0.16681  | 0.1726    | 0.1329   | 0.1973  |
| N7   | -0.59080 | -0.59080  | -0.59080 | -0.59080 | -0.5250   | -0.5854  | -0.5652 |
| C5   | 0.03544  | 0.03544   | 0.03544  | 0.03544  | 0.0226    | -0.2346  | 0.0152  |
| C6   | 0.44911  | 0.51311   | 0.46851  | 0.45811  | 0.5880    | 0.7140   | 0.5597  |
| N6   | -0.30623 | -0.26823  | -0.22923 | -0.25723 | -0.3756   | -0.4189  | -0.4756 |
| H61  | 0.28948  | 0.35948   | 0.38888  | 0.35648  | 0.3306    | 0.3392   | 0.3232  |
| C10  | -0.28897 | -0.29397  | -0.28467 | -0.25597 | -0.3009   | -0.3239  | -0.0774 |
| H101 | 0.12596  | 0.08396   | 0.07536  | 0.09096  | 0.1299    | 0.1400   | 0.0774  |
| H102 | 0.12596  | 0.08396   | 0.07536  | 0.09096  | 0.1299    | 0.1400   | 0.0774  |
| H103 | 0.12596  | 0.08396   | 0.07536  | 0.09096  | 0.1299    | 0.1400   | 0.0774  |
| N1   | -0.67597 | -0.71697  | -0.72167 | -0.72897 | -0.8746   | -0.7617  | -0.6604 |
| C2   | 0.55132  | 0.55132   | 0.55132  | 0.55132  | 0.6898    | 0.5688   | 0.4636  |
| H2   | 0.05539  | 0.05539   | 0.05539  | 0.05539  | 0.0485    | 0.0692   | 0.0865  |
| N3   | -0.73497 | -0.73497  | -0.73497 | -0.73497 | -0.8037   | -0.7900  | -0.7027 |
| C4   | 0.48723  | 0.48723   | 0.48723  | 0.48723  | 0.4807    | 0.6559   | 0.4589  |

Table S2: Charges for all atoms of the m6A nucleobase for different parametrizations.

## S5 Sets of charges

Table S2 shows all the sets of charges considered for the m6A nucleobase. The first column corresponds to the charges from Aduri et al. [1], adjusted to be compatible with the current AMBER force field [2, 3, 4]. Namely, we used the standard AMBER charges for backbone and sugar, and the Aduri et al. charges for the nucleobase. We subtracted  $0.0003 e$  from the charge of each atom so as to maintain the neutral charge of the nucleoside. The following columns represent the charges obtained in our fittings, using: the incorrectly regularized fitting on set A (see Section S4), fit\_A\_inc; the correctly regularized fitting (with  $\alpha = 10$ ) on set A, fit\_A; the correctly regularized fitting (with  $\alpha = 50$ ) on set AB, fit\_AB. In addition, we show charges that we derived following the standard procedure on a nucleobase. We here considered the geometry of both isomers (*syn* and *anti*), computed the electrostatic potentials of the N6-methylated adenine base by Gaussian 09 [7] using the HF/6-31G\* level of theory, subsequently deriving the partial charges via the RESP method [8]. For these calculations we replaced the sugar with a closing methyl group, as done by Aduri *et al.* We notice however that Aduri *et al.* does not report the chosen isomer, which is likely a *syn*, the most populated one for an isolated nucleobase. The last set of parameters (Krepl) have been used in Ref. [9] and were kindly shared by Miroslav Krepl. In order to visualize these sets of charges in a dimensional reduced space, we perform principle components analysis (PCA) on the charges data set, both considering the entire nucleobase (Fig. S6) or only the 6 charges involved in the fitting (Fig. S7). As it can be appreciated in the PCA analysis, the difference by the charges resulting from our fitting procedures and those reported by Aduri is

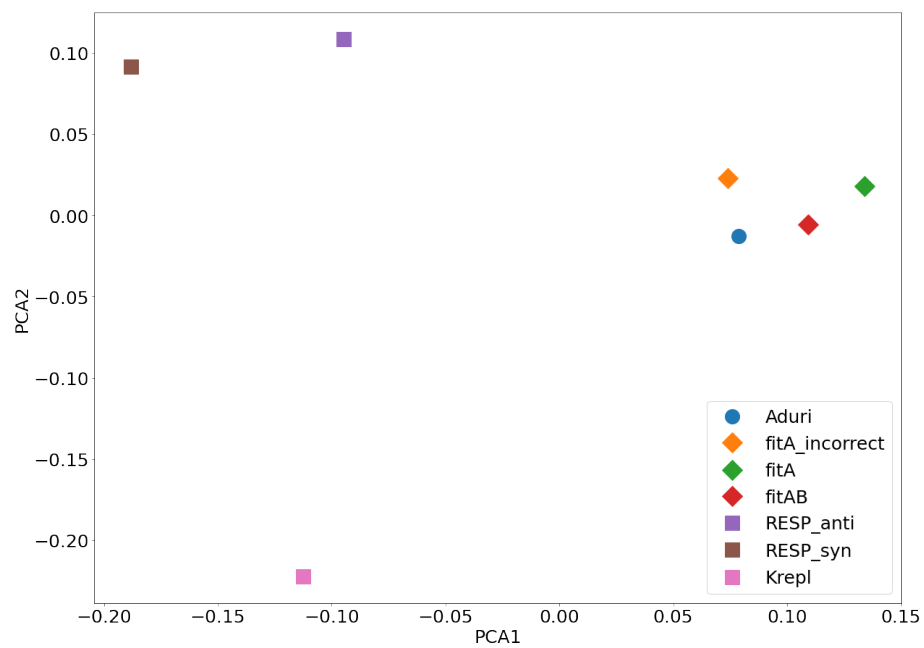

Figure S6: PCA performed giving as input all the charges of the nucleobase.

very small, and significantly lower than the typical variability between different sets of charges obtained with slightly different procedure.

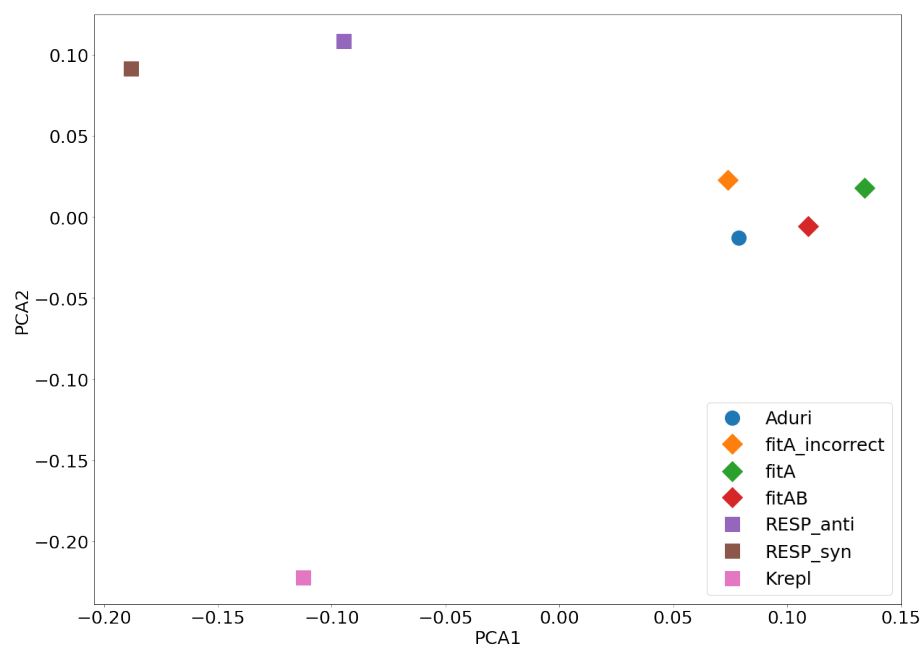

Figure S7: PCA performed giving as input only the 6 charges involved in the fitting.

## S6 Formulas used in the fitting procedure

Our fitting is based on the minimization of a cost function defined as:

$$C = \chi^2 + \alpha \sum_{i=0}^5 \Delta Q_i^2 + \beta V_\eta^2 = \chi^2 + \alpha \left[ \sum_{i=1}^5 \Delta Q_i^2 + \left( \sum_{i=1}^5 \Delta Q_i \right)^2 \right] + \beta V_\eta^2 \quad (4)$$

where  $\alpha$  and  $\beta$  are the hyperparameters needed for regularization of the charges and the torsional term respectively. The  $\chi^2$  measures the discrepancy between computations and experiments:

$$\chi^2 = \frac{1}{N_{exp}} \sum_{i=1}^{N_{exp}} \frac{(\Delta G_{2i-1} - \Delta G_{2i} - \Delta \Delta G_i^{exp})^2}{\sigma_i^2} \quad (5)$$

Alchemical  $\Delta G$ s are computed through a reweighting procedure via the equation:

$$\Delta G^{AFEC} = -k_B T \log \left( \frac{\sum_i^{N_{frame}} w_i e^{-\beta[\Delta E(x_i) + \Delta U(x_i)]}}{\sum_i^{N_{frame}} w_i} \right) \quad (6)$$

where  $w_i$  are the weight derived by the binless WHAM on the original set of energies.  $\Delta U$  correspond to variation in the potential in  $\lambda = 1$  case due to modification of the fitted charges and torsional term:

$$\Delta U(x) = \sum_{i=5}^5 K_i(x) \Delta Q_i + \sum_{i=1}^5 \sum_{j=i}^5 K_{ij}(x) \Delta Q_i \Delta Q_j + V_\eta [1 + \cos(\eta_6(x_i) - \pi)] \quad (7)$$

and  $\Delta E$  is:

$$\Delta E(x_i) = E_{\lambda=1}(x_i) - E_{\lambda=0}(x_i) \quad (8)$$

For the minimization of the cost function through the L-BFGS-B method [10], the derivative of the cost function with respect to the fitted parameters is needed. This should be computed for charges as follows:

$$\frac{\partial C}{\partial \Delta \mathbf{Q}} = \frac{\partial C}{\partial \Delta \mathbf{G}} \frac{\partial \Delta \mathbf{G}}{\partial \mathbf{L}} \frac{\partial \mathbf{L}}{\partial \Delta \mathbf{Q}} \quad (9)$$

Here we introduced the 20-components vector

$$\mathbf{L} = (\Delta Q_1, \Delta Q_2, \dots, \Delta Q_1 \Delta Q_1, \Delta Q_1 \Delta Q_2, \dots, \Delta Q_5 \Delta Q_5) \quad (10)$$

For the torsional parameter instead we have:

$$\frac{\partial C}{\partial V_\eta} = \frac{\partial C}{\partial \Delta \mathbf{G}} \frac{\partial \Delta \mathbf{G}}{\partial V_\eta} \quad (11)$$

The derivative of the free-energy change with respect to  $\mathbf{L}$  components can be computed as

$$\frac{\partial \Delta G_k}{\partial L_l} = \langle K_l \rangle_k = \sum_i^{N_{frame}} w_i K_l^i e^{-\beta[\Delta E(x_i) + \Delta U(x_i) + V_\eta [1 + \cos(\eta_6(x_i) - \pi)]]} \quad (12)$$

|                    | Aduri         |               | Aduri+tors    | fit_A         | fit_AB        |               |
|--------------------|---------------|---------------|---------------|---------------|---------------|---------------|
| method             | BAR           | WHAM          | WHAM+tors     | reweight      | BAR           | WHAM          |
| A1 <i>syn</i>      | 258.24 ± 0.22 | 258.24 ± 0.21 | 258.28 ± 0.21 | 207.76 ± 0.16 | 211.42 ± 0.21 | 211.23 ± 0.18 |
| A1 <i>anti</i>     | 260.12 ± 0.12 | 259.95 ± 0.15 | 264.61 ± 0.15 | 213.12 ± 0.16 | 217.03 ± 0.13 | 217.27 ± 0.19 |
| A2 dup <i>anti</i> | 258.85 ± 0.70 | 258.63 ± 0.33 | 263.29 ± 0.33 | 208.87 ± 0.35 | 214.3 ± 0.7   | 214.01 ± 0.35 |
| A2 dup <i>syn</i>  | 266.44 ± 0.42 | 266.4 ± 0.4   | 266.4 ± 0.4   | 218.87 ± 0.32 | 223.0 ± 0.5   | 222.98 ± 0.34 |
| A2 ss <i>syn</i>   | 257.52 ± 0.31 | 257.54 ± 0.27 | 257.58 ± 0.27 | 204.94 ± 0.44 | 210.34 ± 0.34 | 210.40 ± 0.22 |
| A3 dup <i>anti</i> | 261.56 ± 0.35 | 261.39 ± 0.32 | 266.15 ± 0.32 | 212.18 ± 0.35 | 216.38 ± 0.43 | 216.21 ± 0.38 |
| A3 dup <i>syn</i>  | 267.77 ± 0.35 | 267.75 ± 0.30 | 267.79 ± 0.30 | 216.84 ± 0.31 | 221.96 ± 0.23 | 222.11 ± 0.27 |
| A3 ss <i>syn</i>   | 257.75 ± 0.24 | 257.80 ± 0.32 | 257.84 ± 0.32 | 207.00 ± 0.29 | 211.9 ± 0.5   | 211.17 ± 0.29 |
| A4 dup <i>syn</i>  | 255.06 ± 0.19 | 255.07 ± 0.17 | 255.11 ± 0.17 | 203.54 ± 0.17 | 208.11 ± 0.15 | 208.07 ± 0.17 |
| A4 ss <i>syn</i>   | 257.40 ± 0.19 | 257.42 ± 0.18 | 257.46 ± 0.18 | 207.00 ± 0.19 | 210.56 ± 0.13 | 210.62 ± 0.19 |
| A5 dup <i>syn</i>  | 256.89 ± 0.11 | 256.80 ± 0.19 | 261.76 ± 0.19 | 206.05 ± 0.18 | 209.88 ± 0.16 | 209.93 ± 0.16 |
| A5 ss <i>syn</i>   | 257.56 ± 0.15 | 257.70 ± 0.23 | 257.74 ± 0.23 | 206.93 ± 0.18 | 211.01 ± 0.18 | 210.96 ± 0.16 |
| B1 dup <i>anti</i> | 259.09 ± 0.30 | 259.18 ± 0.21 | 263.94 ± 0.21 | 209.97 ± 0.32 | 213.79 ± 0.35 | 213.81 ± 0.22 |
| B1 ss <i>syn</i>   | 257.73 ± 0.25 | 257.60 ± 0.36 | 257.64 ± 0.36 | 204.84 ± 0.45 | 210.27 ± 0.39 | 210.3 ± 0.6   |
| B2 dup <i>anti</i> | 521.6 ± 0.9   | 521.6 ± 0.9   | 530.9 ± 0.9   | 415.0 ± 0.7   | 434.2 ± 1.0   | 434.1 ± 1.2   |
| B2 ss <i>syn</i>   | 258.34 ± 0.31 | 258.20 ± 0.35 | 258.24 ± 0.35 | 206.82 ± 0.34 | 211.13 ± 0.40 | 211.19 ± 0.29 |
| B3 dup <i>anti</i> | 518.5 ± 1.0   | 518.6 ± 0.9   | 527.9 ± 0.9   | 418.7 ± 0.7   | 430.6 ± 1.4   | 430.5 ± 0.5   |
| B3 ss <i>syn</i>   | 257.74 ± 0.16 | 257.72 ± 0.27 | 257.76 ± 0.27 | 207.2 ± 0.5   | 210.38 ± 0.35 | 210.45 ± 0.22 |
| B4 dup <i>anti</i> | 523.2 ± 1.2   | 523.1 ± 0.5   | 532.4 ± 0.5   | 422.7 ± 0.7   | 433.6 ± 0.9   | 434.8 ± 1.1   |
| B4 ss <i>syn</i>   | 257.84 ± 0.45 | 257.85 ± 0.41 | 257.89 ± 0.41 | 206.6 ± 0.6   | 210.87 ± 0.35 | 210.7 ± 0.5   |
| B5 dup <i>anti</i> | 521.9 ± 0.8   | 522.5 ± 0.7   | 531.8 ± 0.7   | 425.2 ± 0.7   | 434.4 ± 0.9   | 434.4 ± 1.1   |
| B5 ss <i>syn</i>   | 257.04 ± 0.34 | 257.10 ± 0.43 | 257.14 ± 0.43 | 205.75 ± 0.15 | 209.82 ± 0.35 | 209.85 ± 0.19 |

Table S3:  $\Delta G$ s computed through alchemical computations, with different parametrizations and Free Energy methods, reported in  $kJ/mol$ .

The derivative of the free-energy change with respect to the torsional parameter can be computed as

$$\frac{\partial \Delta G_k}{\partial V_\eta} = \langle [1 + \cos(\eta_6(x_i) - \pi)] \rangle_k = \sum_i^{N_{frame}} w_i [1 + \cos(\eta_6(x_i) - \pi)] e^{-\beta[\Delta E(x_i) + \Delta U(x_i) + V_\eta [1 + \cos(\eta_6(x_i) - \pi)]]} \quad (13)$$

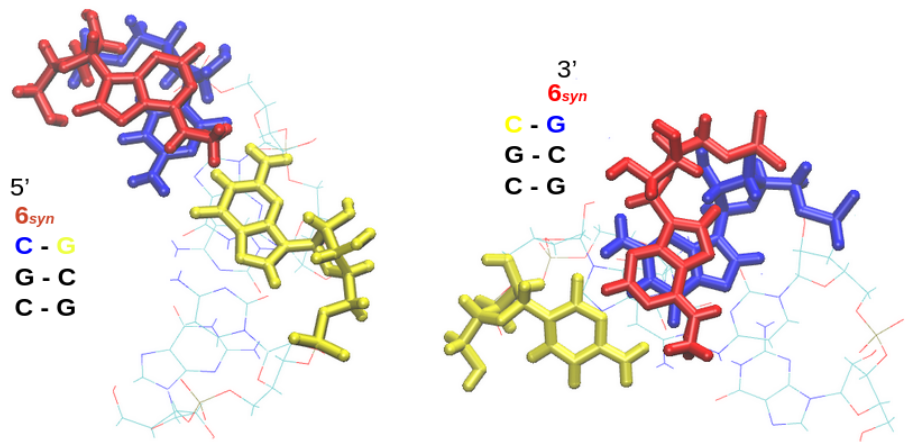

Figure S8: Snapshots from simulations of systems A4 (left) and A5 (right). These are the case where m6A appears as a dangling end and has a stabilization effect on the duplex inducing a favorable stacking. This is due to the hydrophobic screening of the methyl group against adjacent nucleobases. In the A4 case the stabilization effect is greater ( $\Delta\Delta G \sim 2$  kJ/mol) and the methyl group appears in a conformation in which it is covering both neighboring bases from the top, whereas in the A5 case the stabilization is lower ( $\Delta\Delta G \sim 1$  kJ/mol) and the methyl group appears to be shifted to the side.

## S7 Fitting couples of charges

In order to investigate the significance of the fitted parameters, we performed further fittings by tuning only subsets of the parameters. We notice that Aduri charges for N1 and H61, which are involved in Watson Crick pairings with the paired uridine, have partial charge absolute value significantly lower compared to the standard adenine parameters (0.28948 vs 0.41150 for H61, -0.675968 vs. -0.76150 for N1). This may lead to a weakening of hydrogen bonds which may cause an overestimation of destabilization induced on duplexes, as we observed in Aduri+tors cases (see figure 4d in main text). The results of our fitting systematically increase the absolute value of H61 and N1 partial charges, hence resulting in a stronger Watson Crick pairing. At the same time, the torsional term allow to reproduce the correct *anti* isomer penalty. Parameters are coupled, so that it is necessary to fit them simultaneously so as to avoid double counting effects. To demonstrate that N1 and H61 are the most important charges to tune in order to reproduce experiments by strengthening hydrogen bonds, we performed 4 further fittings on the entire data set (AB) by tuning only the torsional plus 2 charges at time, respectively for the couples N1-H61; N1-N6; H61-H101/2/3; N6-H101/2/3, which are taking into account atoms that

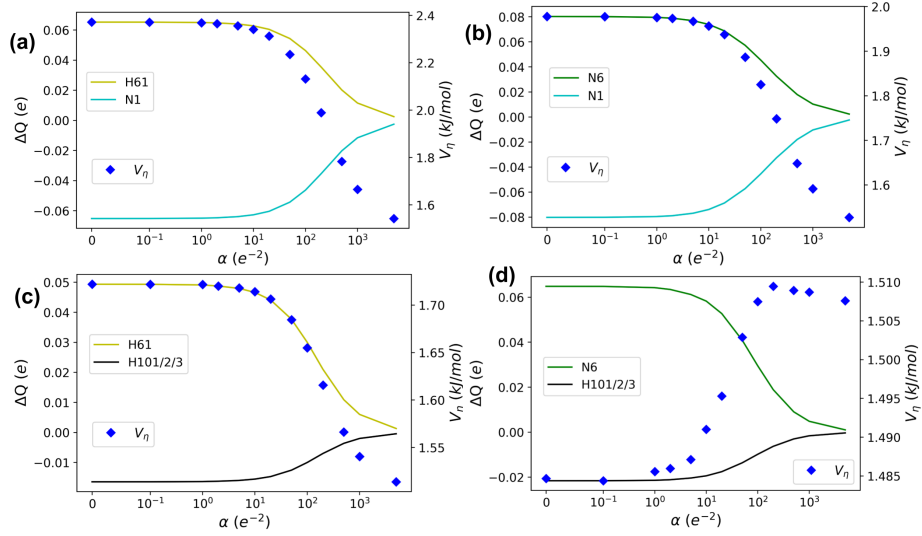

Figure S9: Fitted charges and torsional term  $V_\eta$  as a function of  $\alpha$  ( $\beta = 0$ ). Horizontal axes are in log scale except for 0–0.1 sections which are linear.

have systematic positive and negative  $\Delta Q$  both in fit\_A and fit\_AB. Results are summarized in figure S9.

Interestingly, when fitting only 2 charges, the results are converging for  $\alpha$  going to zero. Furthermore, the Kish Size Ratio obtained for  $\alpha = 0$  is always greater than 0.18, demonstrating that statistical significance is always maintained when fitting only two charges. For  $\alpha$  and  $\beta$  set to zero, results of the fitting are summarized in Table S4.

The lowest  $\chi^2$  is obtained in H61-N1 case with a value of 4.42 (for comparison, the fitted  $\chi^2$  obtained in fit\_AB is 3.61), confirming the hypothesis that tuning these two charges is crucial to reproduce experiments. A slightly larger  $\chi^2$  is obtained in N6-N1 case. Figure S9 also shows that the correction on the torsional angle is highly coupled with modifications of N1 charge. In the two tested cases where N1 was not fitted, the torsional parameter  $V_\eta$  has a smaller dependence on the charges.

|                 | $\Delta Q$ (e) | $V_\eta$ (kJ/mol) | $\chi^2$ | <b>KSR</b> |
|-----------------|----------------|-------------------|----------|------------|
| <b>H61-N1</b>   | 0.0652         | 2.37              | 4.42     | 0.18       |
| <b>N6-N1</b>    | 0.0802         | 1.98              | 4.52     | 0.31       |
| <b>H61-H100</b> | 0.04932        | 1.72              | 5.92     | 0.54       |
| <b>N6-H100</b>  | 0.0648         | 1.49              | 5.93     | 0.74       |

Table S4: Result for fitting 2 charges plus the torsional with hyperparameters set to 0. Only the  $\Delta Q$  associated to the first atom is shown (H61 or N6). The  $\Delta Q$  associated to N1 has the same modulo and opposite sign. The H100 charge is equally distributed on the 3 hydrogens of the methyl group, so that the charge on each hydrogen has 1/3 modulo and opposite sign when compared with the reported  $\Delta Q$ .

|        | fit_AB            |                   |                   |                   |                   |                   | Aduri             |
|--------|-------------------|-------------------|-------------------|-------------------|-------------------|-------------------|-------------------|
| [NaCl] | A1 syn            | A1 anti           | A2 dup            | A2 ss             | A4 dup            | A4 ss             | A2 ss             |
| 0.1 M  | 211.23 $\pm$ 0.18 | 217.27 $\pm$ 0.19 | 214.01 $\pm$ 0.35 | 210.40 $\pm$ 0.22 | 208.07 $\pm$ 0.17 | 210.62 $\pm$ 0.19 | 257.54 $\pm$ 0.27 |
| 1 M    | 212.33 $\pm$ 0.36 | 218.46 $\pm$ 0.25 | 213.99 $\pm$ 0.25 | 210.53 $\pm$ 0.42 | 208.30 $\pm$ 0.33 | 210.91 $\pm$ 0.26 | 257.56 $\pm$ 0.26 |

Table S5:  $\Delta G$ s computed through alchemical computations and binless WHAM method. Each row corresponds to a different NaCl ionic concentrations used in the simulation. Each column correspond so a different system. In the last column, results obtained with the original Aduri parameters are shown as well for one of the systems, confirming that the mild dependence on ion parameters is independent of the precise partial charges used in the simulation.

## S8 Simulations at higher ionic concentration

In this work, the simulations used in the fitting were performed at a ionic concentration of 0.1 M NaCl, which is a value commonly used in molecular dynamics simulations. However, the standard condition in which denaturation experiments, including those analyzed in this work, are performed is 1 M NaCl. In order to quantify the dependence of the computed  $\Delta\Delta G$ s on the ion concentration, we performed further control simulations for a subset of systems at 1 M NaCl. Systems A1, A2 and A4 were chosen in order involve in this checking all possible environments for the methyl group: a nucleoside, where the methyl group is isolated; a duplex with internal m6A, where the methyl group is partly hidden from interactions with ions; a duplex with m6A as a dangling end, where the methyl group is more exposed to interactions with ions; and the corresponding single stranded RNAs, so as to be able to obtain the  $\Delta\Delta G$ s. For the nucleoside, the methylation was added in both *syn* and *anti* conformations. For the other systems, the methylation was added in the expected conformation, as we did for all other systems (see main text).

Results are summarized in Tables S5 and S6. The A1 system, that is the single nucleotide in solution, reports a shift in the  $\Delta G$ s of about 1.2 kJ/mol with respect to 0.1 M cases, for both *syn* and *anti*. As a result, the relative  $\Delta\Delta G$  is not affected. For all other system, the  $\Delta G$ s for the two ionic concentration are in agreement within their statistical error. These results indicate that the fitting is not affected by the discrepancy between the ionic concentration used in computations and experiments.

## S9 List of simulations

We here report the list of simulations performed in this work:

- For the 22 systems reported in Table S3, alchemical simulations were performed using both the Aduri and fit\_AB force-field parameters.
- For 20 of the systems reported in Table S3 (excluding A2\_dup\_syn and A3\_dup\_syn), alchemical simulations were performed using the fit\_A\_incorrect

| [NaCl] | A1              | A2            | A4               |
|--------|-----------------|---------------|------------------|
| 0.1 M  | $6.04 \pm 0.26$ | $3.6 \pm 0.4$ | $-2.55 \pm 0.25$ |
| 1 M    | $6.1 \pm 0.4$   | $3.5 \pm 0.5$ | $-2.6 \pm 0.4$   |
| Exp    | 6.3             | $1.7 \pm 0.9$ | $-2.5 \pm 1.2$   |

Table S6:  $\Delta\Delta G$ s computed through alchemical computations and binless WHAM method. The first two rows correspond to different NaCl ionic concentrations used in the simulation, and last row corresponds to the reference experimental values.

force-field parameters.

- For the 7 systems reported in Table S5, control alchemical simulations were performed at a higher salt concentration.

This resulted in a total of  $22 + 22 + 20 + 7 = 71$  simulations. Each simulation was run with 16 replicas for 10 ns per replicas, for a total simulated time of  $71 \times 16 \times 10\text{ns} = 11.36\mu\text{s}$ .

The size of the simulated systems depended on the number of simulated nucleotides. For the smallest A1 system (one nucleoside), the setup included  $\approx 1500$  water molecules, 3  $\text{Na}^+$  and 3  $\text{Cl}^-$  ions. Double stranded RNAs were simulated in boxes typically containing  $\approx 6000$  water molecules, the largest system being B4 with 7082 water molecules, 32  $\text{Na}^+$  and 14  $\text{Cl}^-$  ions. Single stranded RNAs were simulated using slightly smaller boxes typically containing  $\approx 4500$  water molecules. The smallest systems were A4 and A5, which were solvated in less than 3000 water molecules.

## References

- [1] R. Aduri, B. T. Psciuk, P. Saro, H. Taniga, H. B. Schlegel, and J. SantaLucia. AMBER force field parameters for the naturally occurring modified nucleosides in RNA. *J. Chem. Theory Comput.*, 3(4), 1464–1475, (2007).
- [2] W. D. Cornell, P. Cieplak, C. I. Bayly, I. R. Gould, K. M. Merz, D. M. Ferguson, D. C. Spellmeyer, T. Fox, J. W. Caldwell, and P. A. Kollman. A second generation force field for the simulation of proteins, nucleic acids, and organic molecules. *J. Am. Chem. Soc.*, 117(19), 5179–5197, (1995).
- [3] A. Pérez, I. Marchán, D. Svozil, J. Šponer, T. E. Cheatham III, C. A. Loughton, and M. Orozco. Refinement of the AMBER force field for nucleic acids: improving the description of  $\alpha/\gamma$  conformers. *Biophys. J.*, 92(11), 3817–3829, (2007).
- [4] M. Zgarbová, M. Otyepka, J. Šponer, A. Mládek, P. Banáš, T. E. Cheatham, and P. Jurečka. Refinement of the cornell et al. nucleic acids force field based on reference quantum chemical calculations of glycosidic torsion profiles. *J. Chem. Theory Comput.*, 7(9), 2886–2902, (2011).
- [5] G. Bussi and A. Laio. Using metadynamics to explore complex free-energy landscapes. *Nature Rev. Phys.*, 2(4), 200–212, (2020).
- [6] G. A. Tribello, M. Bonomi, D. Branduardi, C. Camilloni, and G. Bussi. PLUMED 2: New feathers for an old bird. *Comput. Phys. Commun.*, 185(2), 604–613, (2014).
- [7] M. Frisch and et al. Gaussian 09, revision d01. *Gaussian Inc., Wallingford, CT*, (2009).
- [8] P. Cieplak, W. D. Cornell, C. Bayly, and P. A. Kollman. Application of the multimolecule and multiconformational RESP methodology to biopolymers: Charge derivation for DNA, RNA, and proteins. *J. Comput. Chem.*, 16(11), 1357–1377, (1995).
- [9] M. Krepl, F. F. Damberger, C. von Schroetter, D. Theler, P. Pokorná, F. H.-T. Allain, and J. Šponer. Recognition of N6-methyladenosine by the YTHDC1 YTH domain studied by molecular dynamics and NMR spectroscopy: The role of hydration. *J. Phys. Chem. B*, 125(28), 7691–7705, (2021).
- [10] C. Zhu, R. H. Byrd, P. Lu, and J. Nocedal. Algorithm 778: L-BFGS-B: Fortran subroutines for large-scale bound-constrained optimization. *ACM Trans. Math. Softw.*, 23(4), 550–560, (1997).
